# Supplementary material for: Electricity and Reserve Pricing in Chance-Constrained Electricity Markets with Asymmetric Balancing Reserve Policies
Source: arXiv:2106.05999 source file (2021-06-10)
Supplement: Supplementary file 1 [file Appendix.tex]

\begin{comment}
\subsection{Useful derivatives}
\subsubsection{Derivative of \texorpdfstring{\( \soc{A_i\Sigma^{\nicefrac{1}{2}}}^2 \)}{AZ} by \texorpdfstring{$\alpha_{iu}$}{aiu}\label{App: Derivative SOC}}
the term $\soc{A_i\Sigma^{\nicefrac{1}{2}}}^2$ can be expressed as
\begin{IEEEeqnarray}{rl}
    \soc{A_i\Sigma^{\nicefrac{1}{2}}}^2 &= \sum_{u,w} \left[ \alpha_{iu}\alpha_{i,w}\sigma_{u,w} \right] \IEEEyesnumber\IEEEyessubnumber*\\
    &=
    \sum_{u} \left[\alpha_{iu}^2\sigma_{u,u}\right] 
    + \sum_{u, w \ne u} \left[\alpha_{iu}\alpha_{i,w}\sigma_{u,w}\right] \IEEEeqnarraynumspace
\end{IEEEeqnarray}
The first derivative of this expression with respect to $\alpha_{iu}$ yields
\begin{IEEEeqnarray}{rl}
    \IEEEeqnarraymulticol{1}{l}{{\frac{\partial} {\partial \alpha_{iu}}} \left[ \soc{A_i\Sigma^{\nicefrac{1}{2}}}^2 
    \right] \hspace{-1.7cm}}
    \IEEEnonumber \\
    &{=} {\frac{\partial} {\partial \alpha_{iu}}} \left[
    {\sum_{u} \left[\alpha_{iu}^2\sigma_{u,u}\right] 
    {+} \smashoperator{\sum_{u, w \ne u}} \left[\alpha_{iu}\alpha_{i,w}\sigma_{u,w}\right]}
    \right]\IEEEeqnarraynumspace
    \IEEEyesnumber\IEEEyessubnumber*\\
    &{=} 
    2\sum_{u} \left[\alpha_{iu}\sigma_{u,u}\right] 
    {+} 2\smashoperator{\sum_{w \ne u}} \left[\alpha_{i,w}\sigma_{u,w}\right] \label{Eq: der 1 soc SB}\\
    &{=}
    2\smashoperator{\sum_{w}} \left[\alpha_{i,w}\sigma_{u,w}\right] \label{Eq: der final soc SB}
\end{IEEEeqnarray}
The second adding term on \eqref{Eq: der 1 soc SB} follows from the symmetry of the covariance matrix, i.e., $\sigma_{u,w} = \sigma_{w,u}$.
\subsubsection{Derivative of \texorpdfstring{\( \soc{A_i\Sigma^{\nicefrac{1}{2}}}^2 \)}{AZ} by \texorpdfstring{$\widetilde{P}_u$}{Pu} \label{App: Derivative SOC by P_u}}
with $\sigma_u = \kappa_u\widetilde{P}_u$ and $\sigma_{u,v} = \rho_{u,v}\sigma_u\sigma_v$,  the covariance matrix $\Sigma$ is given as:
\begin{subequations}
\begin{IEEEeqnarray}{rCll}
    \Sigma &=& 
        \begin{bmatrix} \sigma_1^2 & \rho_{1,2} \sigma_1 \sigma_2 & \ldots\\
                             \rho_{2,1} \sigma_1 \sigma_2 & \sigma_2^2 & \ldots\\
                             \vdots & \vdots & \ddots 
            \end{bmatrix}\\
    &=& \begin{bmatrix} \kappa_1^2 \tilde{P}_1^2 & \rho_{1,2} \kappa_1 \kappa_2\tilde{P}_1\tilde{P}_2  & \ldots \\
                             \rho_{2,1} \kappa_1 \kappa_2\tilde{P}_1\tilde{P}_2 & \kappa_2^2 \tilde{P}_2^2 & \ldots \\
                             \vdots & \vdots & \ddots 
            \end{bmatrix}
\end{IEEEeqnarray}
\end{subequations}

    
Note that $\rho_{u,v} = \rho_{v,u}$. 
This can be used to take derive the following derivative:
\begin{IEEEeqnarray}{rll}
    \IEEEeqnarraymulticol{1}{l}{{\frac{\partial} {\partial \widetilde{P}_{u}}} \left[ \soc{A_i\Sigma^{\nicefrac{1}{2}}}^2 
    \right] \hspace{-1.7cm}}
    \IEEEnonumber \\
    &{=} {\frac{\partial} {\partial \widetilde{P}_{u}}} \Bigg[
    &\sum_{u} \left[\alpha_{iu}^2\kappa_{u}^2\widetilde{P}^2_u\right] \IEEEnonumber\\
    &&{+} 2\smashoperator{\sum_{u, w \ne u}} \left[\alpha_{iu}\alpha_{i,w}\rho_{u,v}\kappa_{u}\kappa_{v}\widetilde{P}_u\widetilde{P}_v\right]
    \Bigg]\IEEEeqnarraynumspace
    \IEEEyesnumber\IEEEyessubnumber*\\
    &\IEEEeqnarraymulticol{2}{l}{{=}
    2\smashoperator{\sum_{v}} \left[\alpha_{iu}\alpha_{i,v}\rho_{u,v}\kappa_u\kappa_v\widetilde{P}_v \right]} \label{Eq: der final soc SB Pu}
\end{IEEEeqnarray}

\end{comment}

\begin{comment}
\subsection{McCormick Envelopes for Cost Function Relaxation}
\label{sec. McCormick}
To construct convex envelopes for system-wide balancing, we introduce a new variable for every bilinear term \eqref{eq:psi} that is subject to constraints \eqref{eq:mccormick_sw}. This yields feasible solutions, even if those might be sub-optimal. For $\alpha_i$ and $p_i$, the respective upper and lower bounds are required. For $p_i$ these are $\underline{\pmb{P}}_{i},~\overline{\pmb{P}}_{i}$ while for $\alpha_{i(u)}$ we introduce $\underline{\pmb{\alpha}}_{i(u)}, \overline{\pmb{\alpha}}_{i(u)}$. With regards to alpha, we need to consider the system-wide and node-to-node cases. Additionally, constraints
\begin{align}
    \underline{\pmb{\alpha}}_{i(u)} \leq \alpha_{i(u)} \leq \overline{\pmb{\alpha}}_{i(u)},~&\forall~i(,u)\label{eq:alphasapprox}\\
    \underline{\pmb{P}}_{i} \leq p_i \leq \overline{\pmb{P}}_{i},~&\forall~i\label{eq:papprox}
\end{align}
must be imposed, this facilitates control over the approximation quality.
%\vspace{-1ex}
\begin{align}
&\psi_{i} = p_{i}\alpha_{i},~\forall~i\label{eq:psi}\\
&\begin{matrix}
    \psi_{i} \geq \overline{\pmb{\alpha}}_{i}p_{i} + \alpha_{i}\overline{\pmb{P}}_{i} - \overline{\pmb{\alpha}}_{i}\overline{\pmb{P}}_{i}\\
%
    \psi_{i} \leq \overline{\pmb{\alpha}}_{i}p_{i} + \alpha_{i}\underline{\pmb{P}}_{i} - \underline{\pmb{\alpha}}_{i}\overline{\pmb{P}}_{i}\\
%
    \psi_{i} \geq \underline{\pmb{\alpha}}_{i}p_{i} + \alpha_{i}\underline{\pmb{P}}_{i} - \underline{\pmb{\alpha}}_{i}\underline{\pmb{P}}_{i}\\
%
    \psi_{i} \leq \underline{\pmb{\alpha}}_{i}p_{i} + \alpha_{i}\overline{\pmb{P}}_{i} - \underline{\pmb{\alpha}}_{i}\overline{\pmb{P}}_{i}\label{eq:mccormick_sw}\\
\end{matrix},~\forall~i
\end{align}
For node-to-node balancing we define a new matrix or new matrices of variables \eqref{eq:Psi}. For every bilinear term $\Psi_{i,u}$ we impose constraints \eqref{eq:mccormick_n2n}:
%\vspace{-1ex}
\begin{align}
&\Psi_{i} = p_{i} \circ A_{i},~\forall~i\label{eq:Psi}\\
&\begin{matrix}
    \Psi_{i,u} \geq \overline{\pmb{\alpha}}_{iu}p_{i} + A_{i,u}\overline{\pmb{P}}_{i} - \overline{\pmb{\alpha}}_{iu}\overline{\pmb{P}}_{i}\\
%
    \Psi_{i,u} \leq \overline{\pmb{\alpha}}_{iu}p_{i} + A_{i,u}\underline{\pmb{P}}_{i} - \underline{\pmb{\alpha}}_{iu}\overline{\pmb{P}}_{i}\\
%
    \Psi_{i,u} \geq \underline{\pmb{\alpha}}_{iu}p_{i} + A_{i,u}\underline{\pmb{P}}_{i} - \underline{\pmb{\alpha}}_{iu}\underline{\pmb{P}}_{i}\\
%
    \Psi_{i,u} \leq \underline{\pmb{\alpha}}_{iu}p_{i} + A_{i,u}\overline{\pmb{P}}_{i} - \underline{\pmb{\alpha}}_{iu}\overline{\pmb{P}}_{i}\label{eq:mccormick_n2n}\\
\end{matrix},~\forall~i,u.
\end{align}
The full objective function is shown in \eqref{Eq: GCost AB N2N} in its most general form.
Substitution of bilinear terms in $\mathcal{B}$ by $\psi$ and $\Psi$ yields the linear terms ($\hat{\mathcal{B}}$) displayed in Table \ref{tab:objectives}.

{\def\arraystretch{1.25}\tabcolsep=2pt
\begin{table}[ht]
\caption{Bilinear terms in expected costs $\mathbb{E}_{\omega}(c_{i}(p^{2}_{i}))$ for energy markets with system-wide and node-to-node balancing}
\label{tab:objectives}
\begin{center}
\begin{tabular}{|c|cc|}
\hline
& SW & N2N\\
% \midrule
% \multirow{2}{*}{SB} & $\mathcal{B}$ & $-2c_{2,i} p_{i}\alpha_{i} M$ & $-2c_{2,i} p_{i}\alpha_{i}M$\\ & $\hat{\mathcal{B}}$ & $-2c_{2,i}\psi_{i}M$ & $-2c_{2,i}\psi_{i}M$\\
\hline
$\mathcal{B}$ & $-2c_{2,i}p_{i}\alpha_{i}M$ & $-2c_{2,i}p_{i}A_{i}M$\\ 
$\hat{\mathcal{B}}$ & $-2c_{2,i}\psi_{i}M$ & $-2c_{2,i}\Psi_{i}M$\\
\hline
\end{tabular}
\end{center}
\end{table}}

\end{comment}
